# Supplementary material for: Debiasing Embeddings for Reduced Gender Bias in Text Classification
Source: arXiv:1908.02810 source file (2019-08-07)
Supplement: Supplementary file 1 [file xx_Appendix.tex]

\pagebreak

\appendix

\section{Appendices}
\label{sec:appendix}

\begin{table}[h]
\begin{tabular}{lrrrrrrr}
\toprule
  Occupation &  frac\_female & tpr\_F & tpr\_M &  tnr\_F & tnr\_M & tpr\_gap & tnr\_gap \\
\midrule
  dietitian & 0.921 & 0.871 & 0.667 & 0.996 & 0.999 &   0.205 &  -0.004 \\
      nurse & 0.915 & 0.814 & 0.700 & 0.987 & 1.000 &   0.113 &  -0.013 \\
  paralegal & 0.866 & 0.469 & 0.188 & 1.000 & 1.000 &   0.281 &   0.000 \\
      yoga\_teacher & 0.860 & 0.782 & 0.615 & 0.998 & 1.000 &   0.167 &  -0.002 \\
      model & 0.819 & 0.816 & 0.324 & 0.995 & 0.998 &   0.492 &  -0.003 \\
 interior\_designer & 0.784 & 0.589 & 0.333 & 0.999 & 1.000 &   0.256 &  -0.001 \\
      psychologist & 0.621 & 0.718 & 0.698 & 0.989 & 0.994 &   0.020 &  -0.004 \\
    teacher & 0.605 & 0.590 & 0.445 & 0.983 & 0.991 &   0.145 &  -0.009 \\
 journalist & 0.492 & 0.727 & 0.688 & 0.987 & 0.986 &   0.039 &   0.001 \\
  physician & 0.492 & 0.865 & 0.853 & 0.986 & 0.978 &   0.011 &   0.008 \\
       poet & 0.484 & 0.755 & 0.740 & 0.993 & 0.995 &   0.016 &  -0.002 \\
  personal\_trainer & 0.468 & 0.667 & 0.706 & 0.998 & 0.999 &  -0.040 &  -0.001 \\
  professor & 0.452 & 0.911 & 0.913 & 0.934 & 0.937 &  -0.003 &  -0.003 \\
    painter & 0.452 & 0.773 & 0.752 & 0.996 & 0.996 &   0.021 &   0.000 \\
 accountant & 0.375 & 0.657 & 0.736 & 0.999 & 0.998 &  -0.079 &   0.001 \\
   attorney & 0.367 & 0.883 & 0.893 & 0.989 & 0.990 &  -0.011 &  -0.001 \\
      photographer & 0.357 & 0.881 & 0.910 & 0.985 & 0.983 &  -0.029 &   0.002 \\
    dentist & 0.346 & 0.949 & 0.937 & 0.998 & 0.996 &   0.012 &   0.001 \\
  filmmaker & 0.322 & 0.815 & 0.833 & 0.997 & 0.994 &  -0.018 &   0.003 \\
      chiropractor & 0.298 & 0.559 & 0.602 & 0.999 & 0.999 &  -0.043 &   0.000 \\
     pastor & 0.231 & 0.583 & 0.699 & 0.998 & 0.996 &  -0.116 &   0.002 \\
  architect & 0.225 & 0.661 & 0.614 & 0.996 & 0.992 &   0.047 &   0.004 \\
   comedian & 0.221 & 0.735 & 0.820 & 0.999 & 0.996 &  -0.086 &   0.002 \\
 software\_engineer & 0.157 & 0.732 & 0.736 & 0.998 & 0.990 &  -0.004 &   0.008 \\
    surgeon & 0.154 & 0.469 & 0.671 & 0.998 & 0.992 &  -0.202 &   0.006 \\
   composer & 0.153 & 0.744 & 0.792 & 0.999 & 0.997 &  -0.048 &   0.002 \\
  dj & 0.145 & 0.647 & 0.645 & 0.999 & 0.998 &   0.002 &   0.001 \\
     rapper & 0.086 & 0.765 & 0.812 & 0.999 & 0.997 &  -0.047 &   0.002 \\
\bottomrule
\end{tabular}
\caption{Detailed metrics for the GloVe model}
\end{table}

\section{Supplemental Material}
\label{sec:supplemental}
